# Supplementary material for: Discrimination in the Venture Capital Industry: Evidence from Field Experiments
Source: arXiv:2010.16084 source file (2022-08-14)
Supplement: Supplementary file 1 [file appendix_estimator.tex]

%Backup

\begin{table}
 \caption{Experiment A Implicit Discrimination Based on Founder's Gender by Investors' Industry}
  \label{implicit bias gender industry}
 \begin{center}
 \scalebox{0.85}{
\begin{tabular}{l c c c c c} 
\toprule
Dependent Variable&Response Time&Q1&Q2&Q3&Q4\\
&(Unit: Second)&Profitability&Availability&Contact&Investment\\
&(1)&(2)&(3)&(4)&(5)\\
\midrule
\emph{Panel A: Tech Sector Investors}&&&&&\\
&&&&&\\
Second Half of Study&-24.87***&	2.96&4.63***&-0.56&	1.18***\\
&(2.81)&(2.11)&	(1.70)&	(2.63)&	(0.38)\\
Female Founder&1.28&2.73&1.71&	-0.16&	0.53\\
&(2.82)&(2.16)&	(1.78)&	(2.62)&	(0.38)\\
Female Founder $\times$&&-6.59**&-3.28&-3.87&-1.21**\\
Second Half of Study&&(3.16)&(2.47)&(3.83)&	(0.56)\\
&&&&&\\
Investor FE &Yes&Yes&Yes&Yes&Yes\\
Observations&784&784&752&784&774\\
R-squared&0.31&0.31&0.41&0.41&0.33\\
&&&&&\\
\emph{Panel B: Non-tech Sector Investors}&&&&\\
&&&&&\\
Second Half of Study&-31.58***&	1.49&-1.88&	3.56&0.51\\
&(3.92)&(2.53)&	(1.74)&	(2.79)&	(0.45)\\
Female Founder&-6.30&-0.41&	0.38&3.03&0.59\\
&(3.97)&(2.71)&	(1.94)&	(3.10)&	(0.49)\\
Female Founder $\times$&&-0.24&	1.21&-3.48&	-0.69\\
Second Half of Study&&(3.69)&(2.41)&(4.02)&	(0.65)\\
&&&&&\\
Investor FE &Yes&Yes&Yes&Yes&Yes\\
Observations&432&432&432&432&402\\
R-squared&0.37&	0.30&0.71&0.54&	0.38\\
\bottomrule
\end{tabular}}
\end{center}
\begin{tablenotes}
\item \footnotesize \emph{Notes.} This table reports regression results of how the response time and evaluation results of investors from different industries respond to a startup founder's gender. Panel A tests the implicit gender discrimination of investors working in the tech sectors (i.e., IT, cyber security, software, etc.). Panel B tests the implicit gender discrimination of investors working in non-tech sectors (i.e., media, entertainment, education, etc.). ``Female Founder" is a dummy variable that is equal to one if the startup founder has a female first name, and zero otherwise. ``Second Half of Study" is an indicator variable for startup profiles shown among the last half profiles viewed by a subject. In column (1), the dependent variable is investors' response time, which is defined as the number of seconds before each page submission, winsorized at the $95^{th}$ percentile (59.23 seconds on average). Columns (2)-(5) show the profitability evaluation, availability evaluation, contact interest ratings, and investment interest ratings, respectively. Standard errors in parentheses are clustered at the investor level. ***$p<0.01$, **$p <0.05$, *$p<0.1$
\end{tablenotes}
\end{table}

%%%%%%%%%%%%%%%%%%%%
%%%Evaluation (Team & Project)%%%
%%%%%%%%%%%%%%%%%%%%
\clearpage
\begin{center}
\begin{table}
\caption{Evaluation Results of Other Startup Characteristics in Experiment A}
\label{irr_teamproject}
\scalebox{0.85}{ 
\begin{tabular}{l c c c c c c c} 
\toprule
Dependent Variable&Q1&Q2&Q3&Q3&Q4&Q4&Q5\\
&Profitability&Availability&Contact&Contact&Investment&Investment&Risk\\
&(1)&(2)&(3)&(4)&(5)&(6)&(7)\\
\midrule
Serial Founder&5.23***&	-0.81&	5.64***&	1.26&	0.76***&	0.13&	-0.65\\
&(1.08)&	(0.88)&	(1.28)&	(0.91)&	(0.19)&	(0.15)&	(3.05)\\
Ivy&5.36***&	-1.06&	7.44***&	3.01***&	0.87***&	0.20&	-6.44**\\
&(1.10)&	(0.87)&	(1.31)&	(0.93)&	(0.20)&	(0.15)&	(3.26)\\
Number of Founders&1.56&	-1.21&	1.17&	-0.11&	0.21&	0.04&	-5.32*\\
&(1.07)&	(0.88)&	(1.29)&	(0.91)&	(0.20)&	(0.15)&	(3.06)\\
US Founder	&0.95&	0.02&	4.23***&	3.69***&	0.08&	0.03&	-0.91\\
&(1.18)&	(0.91)&	(1.39)&	(1.00)&	(0.21)&	(0.16)&	(3.48)\\
\# Comparative Adv&3.10***&	-0.22&	2.76***	&0.34&	0.55***	&0.15**&	0.91\\
&(0.54)&	(0.43)&	(0.64)&	(0.43)&	(0.10)&	(0.07)&	(1.48)\\
Has Positive Traction&12.70***&	1.75**&	13.35***&	1.91*&	1.81***&	0.28*&	-9.51***\\
&(1.07)	&(0.86)&	(1.28)&	(0.99)&	(0.20)&	(0.16)&	(3.15)\\
Number of Employees [0-10]&0.67	&2.37**	&-1.73&	-2.57**&	-0.19&	-0.29&	-1.18\\
&(1.43)&	(1.16)&	(1.69)&	(1.18)&	(0.26)&	(0.20)&	(3.94)\\
Number of Employees [10-20]&-1.08&	0.94&	-3.26&	-2.08&	-0.46&	-0.33	\\
&(1.64)&	(1.35)&	(1.99)&	(1.39)&	(0.30)&	(0.23)\\
Number of Employees [20-50]&-0.47&	-0.02&	-1.21&	-0.72&	-0.16&	-0.12&	-1.28\\
&(1.45)&	(1.17)&	(1.71)&	(1.17)&	(0.27)&	(0.19)&	(3.59)\\
Company Age&-4.59*&	-5.99***&	-7.39**&	-2.19&	-1.26**&	-0.54&	-3.41\\
&(2.72)&	(2.19)&	(3.19)&	(2.26)&	(0.49)&	(0.37)&	(7.74)\\
Company Age$^2$	&0.75&	1.12**&	1.27**&	0.42&	0.23**&	0.10&	0.77\\
&(0.54)&	(0.44)&	(0.64)&	(0.45)&	(0.10)&	(0.07)&	(1.52)\\
Is B2B&	3.90***	&3.73***&	6.10***	&1.47&	0.81***&	0.32**	&-4.91\\
&	(1.07)&	(0.86)&(1.28)&	(0.89)&	(0.20)&	(0.15)&	(3.01)\\
Domestic Market&-0.10&	-0.60&	0.09&	0.57&	0.08&	0.13&	-3.32\\
	&(1.08)&	(0.86)&	(1.28)&	(0.90)&	(0.20)&	(0.14)&	(3.19)\\

Q1	&&&&		0.88***		&&	0.12***	\\
	&&&&			(0.03)		&&(0.01)\\
Q2	&&&&			0.18***		&&0.01\\
		&&&&		(0.03)	&&	(0.01)\\
					
Constant&49.75***&	78.20***&	66.20***&	-4.19&	5.62***&	-0.33&	67.01***\\
&(6.56)&	(6.02)&	(4.93)&	(7.50)&	(1.43)&	(0.63)&	(11.66)\\
 &&&&&&\\
Investor FE &Yes&Yes&Yes&Yes&Yes&Yes\\
Observations&	1,216&	1,184&	1,216&	1,184&	1,176&	1,154&	176\\
R-squared&	0.44&	0.55&	0.56&	0.80&	0.44&	0.70&	0.34\\
\bottomrule

\end{tabular}}
 \begin{tablenotes}

\item\footnotesize \emph{Notes.} This table shows that investors understand the incentives and care about multiple important startup team and project characteristics. In columns (1)-(7), the dependent variable is the evaluation results of Q1 (profitability evaluation), Q2 (collaboration interest), Q3 (contact interest),  Q3 (contact interest), Q4 (contact interest), Q4 (investment interest), and Q5 (risk evaluation). ``Serial Founder," ``Ivy," ``US Founder," ``Has Positive Traction," ``Is B2B," and ``Domestic Market" are indicative variables that equal to one if the founder is a serial entrepreneur, graduates from an Ivy League college, or lives in the U.S., and the project has positive traction, is a business-to-business startup, or focuses on the domestic market. These variables are equal to 0 if the startup does not have such characteristics. ``Number of founders" is either 1 or 2; ``Number of Comparative Advantages" and ``Company Age" can be \{1,2,3,4\}; ``Company Age$^2$" is the square of the company age. ``Q1" is the evaluation results of startup profitability. ``Q2" is the evaluation results of the collaboration likelihood. All the regression results add investor fixed effect and use the robust standard errors reported in parentheses. I use the Bonferroni method to implement multiple hypothesis testing. *** p$<$0.01, ** p$<$0.05, * p$<$0.1

\end{tablenotes}
\end{table}
\end{center}

%%%%%%%%%%%%%%%%%%%%%%%%%%%%%%%%%%%%%%%%%%%%%%%%%%%%%%%%%%%%%
%%%%%%% Quantile Regression (Gender) First Half %%%%%%%%%%%%%
%%%%%%%%%%%%%%%%%%%%%%%%%%%%%%%%%%%%%%%%%%%%%%%%%%%%%%%%%%%%%

\begin{sidewaystable}
\begin{center} 
\caption{Quantile-Regression Estimates for Investors' Evaluations (First-half of Study, Gender)}
\label{irr_investor_profile_gender_quantile_first}
\scalebox{0.9}{
\begin{tabular}{ m{5cm} c c c c c c c c c c}
&&&&&&&&&&\\
\toprule 
&10th&20th&30th&40th&50th&60th&70th&80th&90th&Mean\\
&[1]&[2]&[3]&[4]&[5]&[6]&[7]&[8]&[9]&[10]\\
\midrule
\emph{Panel A. Tech Sector}&&&&&&&&&&\\
&&&&&&&&&&\\
Female Founder&3.00&5.00&0.00&0.00&0.00&4.00&0.00&3.00&0.00&0.22\\
&(3.97)&(4.43)&(5.23)&(6.72)&(5.98)&(4.41)&(4.07)&(3.67)&(1.64)&(2.72)\\
Quantile of Dep. Var.&5&17&25&40&50&65&75&80&100&51.02\\
&&&&&&&&&&\\
Observations&392&392&392&392&392&392&392&392&392&392\\
&&&&&&&&&&\\
&&&&&&&&&&\\
\emph{Panel B. Full Sample}&&&&&&&&&&\\
&&&&&&&&&&\\
Female Founder&4.00&1.00&5.00&1.00&5.00&3.00&0.00&0.00&0.00&1.30\\
&(3.61)&(4.21)&(4.73)&(5.44)&(3.90)&(3.90)&(3.58)&(2.80)&(0.87)&(2.07)\\
Quantile of Dep. Var.&10&20&31&50&60&70&80&90&100&55.20\\
&&&&&&&&&&\\
Observations&608&608&608&608&608&608&608&608&608&608\\
\bottomrule
\end{tabular}}
 \end{center}
\begin{tablenotes}
\item \footnotesize \emph{Notes.} This table reports the effects of a startup founder's gender on the quantiles and the mean of investors' contact interest ratings (i.e., $Q_3$) of the first half of the experiment. In each of Columns [1]–[9], the dependent variable is the $k$th percentile ($k\in{10,20,...,90}$) of the distribution of the startup's perceived attractiveness measured by investors' contact interest ratings (i.e., $Q_3$). In Column [10], the dependent variable is the average investor's contact interest ratings of the first half profiles. Panel A focuses on the evaluation results of investors working in the tech sector. Panel B uses the evaluation results of all recruited investors. Standard errors in parentheses are clustered at the investor level. $*p < 0.10, **p < 0.05, ***p < 0.01$\\
\end{tablenotes}
\end{sidewaystable}

%%%%%%%%%%%%%%%%%%%%%%%%%%%%%%%%%%%%%%%%
%%%%%%% Quantile Regression (Race) %%%%%%%%%%%
%%%%%%%%%%%%%%%%%%%%%%%%%%%%%%%%%%%%%%%%

\begin{sidewaystable}
\begin{center} 
\caption{Quantile-Regression Estimates for Investors' Evaluations (First-half of Study, Race)}
\label{irr_investor_profile_race_quantile_first}
\scalebox{0.9}{
\begin{tabular}{ m{5cm} c c c c c c c c c c}
&&&&&&&&&&\\
\toprule 
&10th&20th&30th&40th&50th&60th&70th&80th&90th&Mean\\
&[1]&[2]&[3]&[4]&[5]&[6]&[7]&[8]&[9]&[10]\\
\midrule
\emph{Panel A. Tech Sector}&&&&&&&&&&\\
&&&&&&&&&&\\
Asian Founder&-1.00&5.00&4.00&0.00&0.00&2.00&0.00&1.00&0.00&-0.64\\
&(3.64)&(4.18)&(5.01)&(5.99)&(5.53)&(4.49)&(4.95)&(4.76)&(1.67)&(3.21)\\
Quantile of Dep. Var.&5&17&25&40&50&65&75&80&100&51.02\\
&&&&&&&&&&\\
Observations&392&392&392&392&392&392&392&392&392&392\\
&&&&&&&&&&\\
&&&&&&&&&&\\
\emph{Panel B. Full Sample}&&&&&&&&&&\\
&&&&&&&&&&\\
Asian Founder&-1.00&0.00&1.00&-8.00*&-6.00&0.00&0.00&0.00&0.00&-0.63\\
&(3.24)&(4.21)&(5.20)&(4.49)&(4.22)&(4.15)&(4.16)&(2.78)&(0.94)&(2.57)\\
Quantile of Dep. Var.&10&20&31&50&60&70&80&90&100&55.20\\
&&&&&&&&&&\\
Observations&608&608&608&608&608&608&608&608&608&608\\
\bottomrule
\end{tabular}}
\end{center}
\begin{tablenotes}
\item \footnotesize \emph{Notes.} This table reports the effects of a startup founder's race on the quantiles and the mean of investors' contact interest ratings (i.e., $Q_3$) of the first half of the experiment. In each of Columns [1]–[9], the dependent variable is the $k$th percentile ($k\in{10,20,...,90}$) of the distribution of the startup's perceived attractiveness measured by investors' contact interest ratings (i.e., $Q_3$). In Column [10], the dependent variable is the average investor's contact interest ratings of the first half profiles. Panel A focuses on the evaluation results of investors working in the tech sector. Panel B uses the evaluation results of all recruited investors. Standard errors in parentheses are clustered at the investor level. $*p < 0.10, **p < 0.05, ***p < 0.01$\\
\end{tablenotes}
\end{sidewaystable}

\begin{figure}
    \centering
    \includegraphics[scale=0.55]{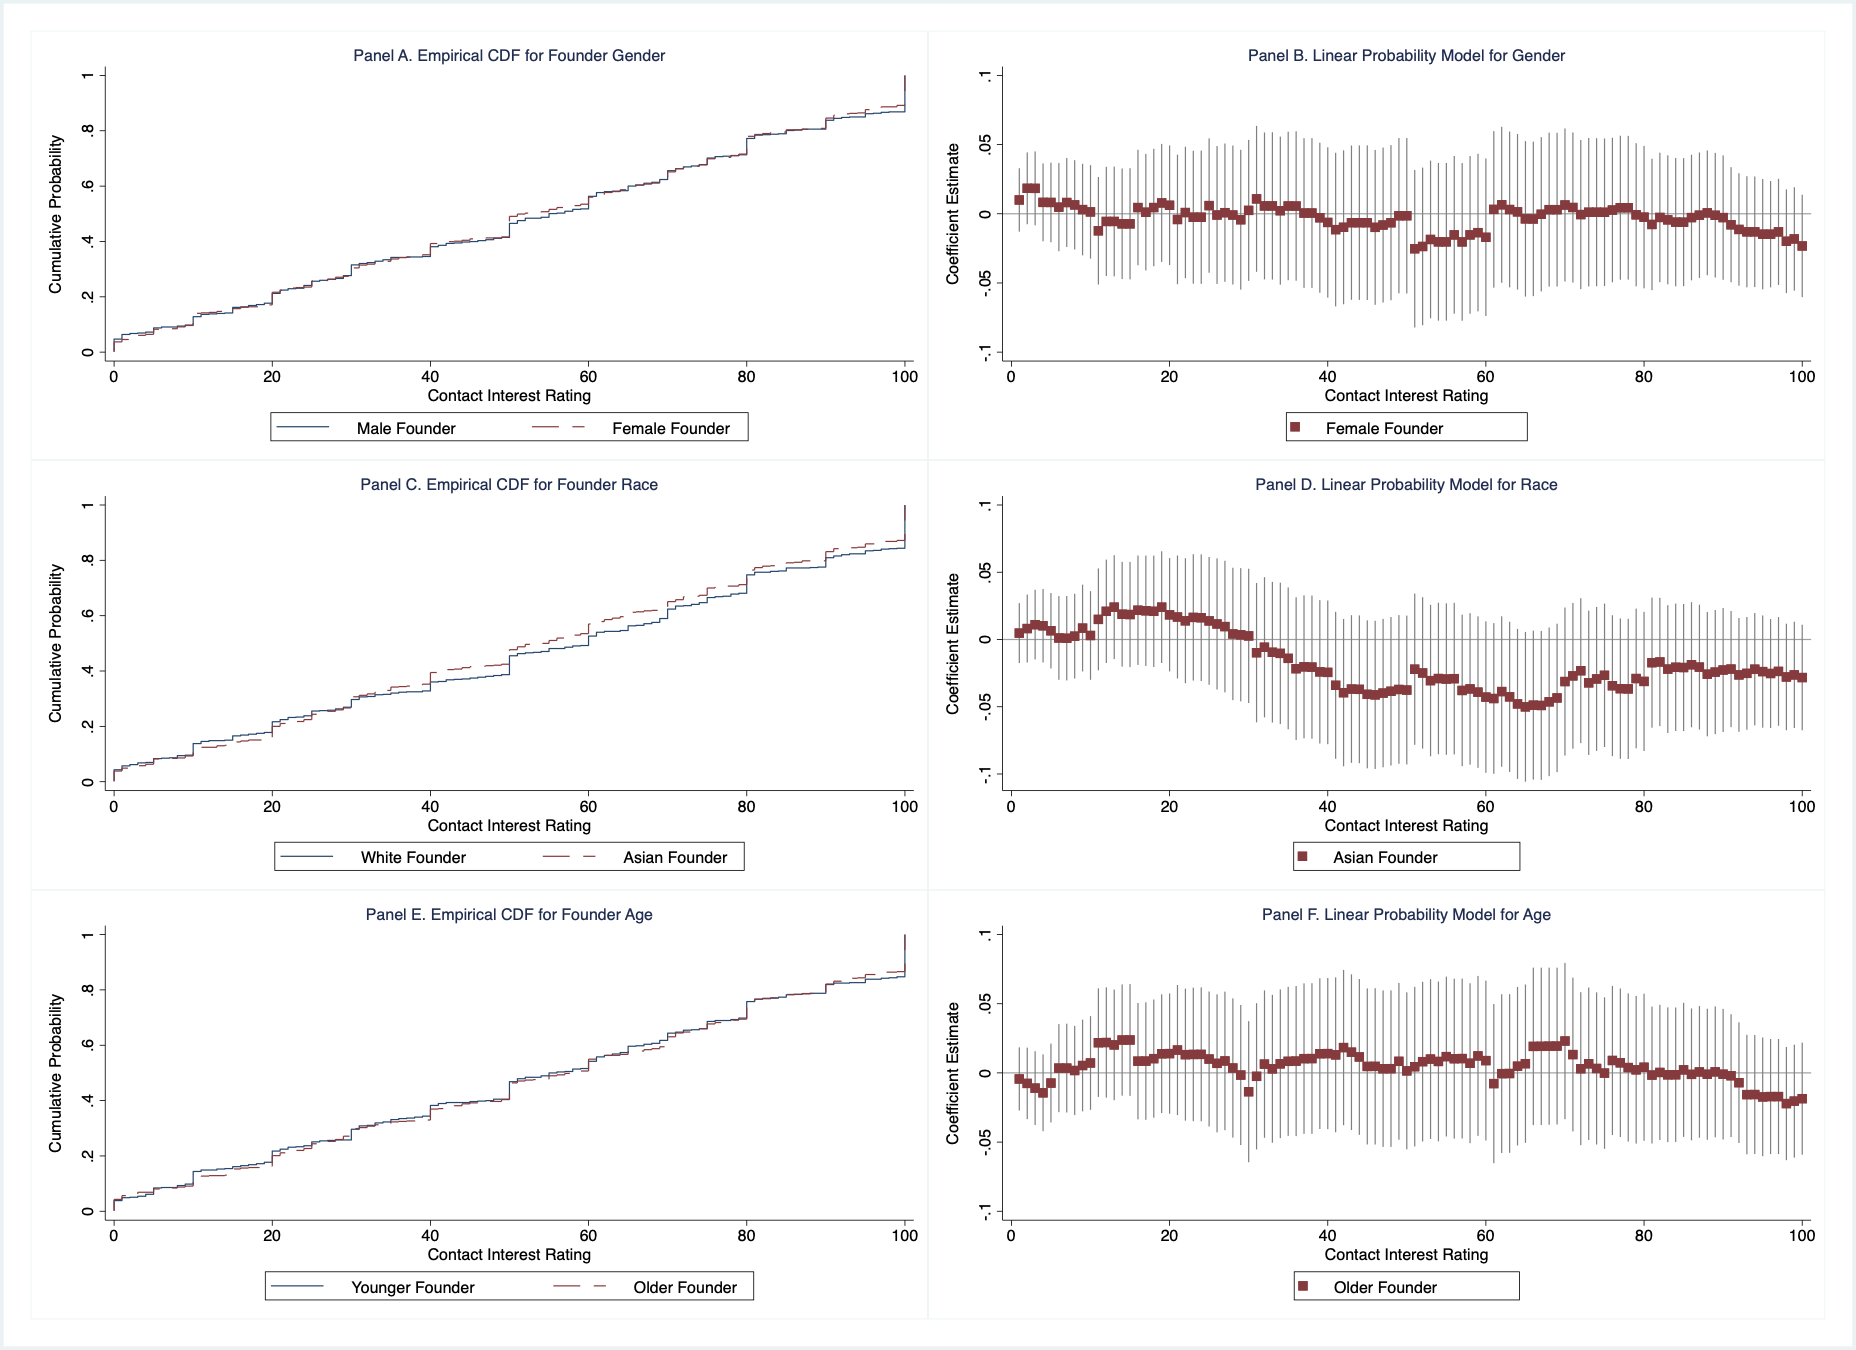}
     \caption{Gender, Racial, and Age Discrimination across Contact Interest Ratings (Total Profiles)}
    \captionsetup{labelformat=empty}
    \caption*{\footnotesize \emph{Notes}: This figure demonstrates the effect of a startup founder's gender, race, and age across the contact interest distribution using the total profiles evaluated in Experiment A. Panel A provides the empirical CDF for a founder's gender on investors' contact interest rating (i.e. $Pr(\text{Contact Interest}\leq x|\text{Female Founder})$ and $Pr(\text{Contact Interest}\leq x|\text{Male Founder})$). Panel B provides the OLS coefficient estimates (i.e. $Pr(\text{Contact Interest}\leq x|\text{Female Founder})-Pr(\text{Contact Interest}\leq x|\text{Male Founder}))$ and the corresponding 95\% confidence level. Similarly, Panels C and E provide the empirical CDF for a founder's race and age. Panels D and F provide the OLS coefficient estimates for a founder's race and age.}
     \label{fig:distribution_total}
\end{figure}

\clearpage
\begin{table}
 \caption{Experiment B Robustness Check of Heterogeneous Effect of Investors' Response (ESG)}
 \label{table_ESG2}
 \begin{center} 
 \scalebox{0.85}{ 
\begin{tabular}{l c c c c c c } 
\toprule
&&&&&&\\
& \multicolumn{6}{c}{Dependent Variable: \textbf{$1$}(\emph{Opened}) }\\
\cline{2-7}
&(1)&(2)&(3)&(4)&(5)&(6)\\
&Full&Impact Fund&Common Fund&Full&Impact Funds&Common Fund\\
\midrule
Female Founder=1&0.009**&0.023*	&0.009**&&&\\
&(0.004)&(0.013)&(0.004)&&&\\
Asian Founder=1&&&&0.008&-0.022&0.008\\
&&&&(0.005)&(0.019)&(0.005)\\
Impact Fund=1&0.014&&&0.039***&&\\
&(0.010)&&&(0.015)&&\\
&&&&&&\\
Female Founder=1 $\times$&0.014&&&&&\\
Impact Fund=1&(0.014)	&&&&&\\
&&&&&&\\
Asian Founder=1 $\times$&&&&-0.029	&&\\
Impact Fund=1&&&&(0.020)	&&\\
&&&&&&\\
US Investor=1&-0.015**&	-0.044**&	-0.010&	-0.027***&	-0.056**&	-0.022***\\
&	(0.006)&	(0.018)&	(0.007)&	(0.008)&	(0.023)	&(0.008)\\
Female Investor=1&-0.021***	&-0.030*&	-0.019***&	-0.015**&	-0.017&	-0.015**\\
&	(0.005)	&(0.016)&	(0.005)&	(0.006)	&(0.020)&	(0.006)\\
Constant&0.190***&	0.237***&	0.184***&	0.143***&	0.144**&	0.146***\\
&	(0.019)	&(0.054)&	(0.020)	&(0.019)&	(0.061)&	(0.019)\\
&&&&&&\\
Startup FE&Yes&Yes&Yes&Yes&Yes&Yes\\
Observations&	30,909&	2,895&	28,014	&14,348	&1,335	&13,013\\
R-squared&0.006&0.014&	0.006&	0.006&	0.012&	0.006\\
\bottomrule
\end{tabular}}
\end{center}
\begin{tablenotes}
\item \footnotesize
\emph{Notes.} This table reports the heterogeneous effect of global investors' email opening behaviors based on their investment philosophies in the correspondence test. The definition of impact funds is more general, including both non-profit funds and funds whose description contains suggestive keywords. The dependent variable is a dummy variable, which is one when an investor opens the pitch email, and zero otherwise. ``Female Founder = 1" is an indicator variable that equals one if the first name of the email sender is a female name, and zero otherwise. Similarly, ``Asian Founder =1" is an indicator variable that equals one if the last name of the email sender is an East Asian name, and zero otherwise. ``Impact Fund=1" is an indicator variable that equals one if the investor works in a fund with ESG-related investment preferences based on Pitchbook Data, and zero otherwise. Such preferences include supporting minority founders, caring about the environmental and social impact, etc. ``US Investor =1" and ``Female Investor = 1" are indicator variables for being a U.S. investor and being a female investor. Columns (1) and (4) report the regression results for all observations with available investment philosophies. Columns (2) and (5) report the regression results for investors working in impact funds. Columns (3) and (6) report the regression results for investors working in common VC funds which do not pursue impact investing strategies. $R^2$ is the adjusted $R^2$ for OLS regressions. Standard errors are in parentheses and are clustered at the investor level. *** p$<$0.01, ** p$<$0.05, * p$<$0.1
\end{tablenotes}
\end{table}

\clearpage
\begin{sidewaystable}
\caption{Bias Mechanisms Predicted by Theories (Gender)}
\begin{center} 
\label{cor:mechanismgender}
\scalebox{0.85}{
\small
%\begin{tabular}{ m{7cm}  m{2cm} m{4.8cm} m{2cm} m{4.5cm}} 
\begin{tabular}{ m{8cm}  m{2cm} m{5cm} m{2cm} m{4cm}} 
&&&&\\
\toprule
Mechanisms&Experiment A&Theory Prediction&Experiment B&Theory Prediction\\
\midrule
\textbf{1. Belief-Based Mechanisms}&&&&\\
\midrule
1.1 Expected financial return (first moment)&$\surd$ \textcolor{red}{(against)}&Q1, $\beta_{female}\neq0$&$\varnothing$&$\beta_3<0$\\
1.2 Expected variation (second moment)&$\times$&Q5, $\beta_{female}\neq0$&$\times$&$\sigma_{FR}^{II}\neq1$\\
1.3 Strategic channel&$\times$&Q2, $\beta_{female}\neq0$&$\times$&$\beta_2<0$\\
\midrule
\textbf{2. Taste-Based
Mechanisms}&&&$\surd$&$\beta_1>0,\beta_2>0,\beta_3>=0$\\
\midrule
2.1 Friendly Support&$\surd$&Female investors donate more to female founders.&$\surd$&$\beta_1$ is larger for impact funds\\
2.2 Social Image&$\varnothing$-$\surd$&Male investors donate less to female founders in the donation game&$\varnothing$&\\
2.3 Others (i.e. Sexual harassment)&$\varnothing$&Older female founders are less likely to be contacted.&$\varnothing$&\\
\midrule
\textbf{Amplifying Mechanisms}&&&&\\
\midrule
a. Attention Discrimination&$\varnothing$&&$\surd$&$\beta_1>0$ when $Y_{ij}$ is opening rates and email staying time.\\
b. Implicit Bias&\textcolor{red}{$\surd$ (against)}&Test interaction term of Female Founders and the Second Half Study&$\varnothing$& \\
\midrule
\textbf{3. Other Specific Mechanisms}&&&&\\
\midrule
3.1 Uninformative Email Behaviors&N/A&&$\times$&$\beta_1>0$ when $Y_{ij}$ is opening rates and email staying time.\\
3.2 Fishy Emails&N/A&&$\times$&$\beta_2<0$\\
\bottomrule
\end{tabular}}
 \end{center}
 \begin{tablenotes}
\item \footnotesize \emph{Notes.} This table shows the mechanisms predicted by different gender discrimination theories and whether such mechanisms are supported by the empirical results from the correspondence test and the lab-in-field experiment or not. ``$\surd$" means such a mechanism is supported by the empirical evidence from the specific experiment. ``$\times$" means that such a mechanism is ruled out by the empirical evidence from the specific experiment. ``$\varnothing$" means that the experiment does not provide empirical evidence to support or rule out such a mechanism. The parameters used in the correspondence test theory predictions are from the following regressions: $Y_{ij}=\beta_0+\beta_1 FemaleFounder{ij}+\beta_2 Ivy_{ij}+\beta_3 FemaleFounder_{ij}\times Ivy_{ij}+\alpha_i +\epsilon_{ij}$ with pitch email fixed effect, where $Y_{ij}$ are the behavior measurements like the opening rate dummy, etc. $FemaleFounder_{ij}$ and $Ivy_{ij}$ are indicators of being a female founder and graduating from Ivy League colleges. $\sigma_{FR}^{II}$ is the ratio of standard errors of female founders' unobservable characteristics and male founders' unobservable characteristics. I found bias towards female founders ($\beta_1>0$) in the correspondence test. Hence, all the theory predictions are to explain the reasons why investors prefer female founders. The parameters used in the lab-in-field theory predictions are from the following regressions: $V_{ij}=\beta_0+\beta_c Characteristics_{ijc}+\alpha_i+\epsilon_{ij}$ with evaluator fixed effect.$V_{ij}$ can be the evaluation of Q1(quality), Q2(collaboration likelihood), Q3(contact), Q4(investment) and Q5(risk). Please note that all the mechanisms can exist at the same time with some mechanisms dominating others in specific experimental settings.
\end{tablenotes}
\end{sidewaystable}

%%%%%%%%%%%%%%%%%%%%%%%%%%%%%%%%%%%%%%%%%%%%%%%%%%%%%%%%%%
\clearpage
\begin{sidewaystable}
\caption{Bias Mechanisms Predicted by Theories (Race)}

\label{cor:mechanismrace}
%\begin{tabular}{ m{4cm} m{2cm} m{3cm} m{2cm} m{4cm}}
\begin{center} 
\scalebox{0.9}{ 
\small
\begin{tabular}{ m{8cm}  m{2cm} m{5cm} m{2cm} m{4cm}}
&&&&\\
\toprule 
Mechanisms&Experiment A&Theory Prediction&Experiment B&Theory Prediction\\
\midrule
\textbf{1. Belief-Based Mechanisms}&&&&\\
\midrule
1.1 Expected financial return (first moment)&\textcolor{red}{$\surd$ (against)}&Q1, $\beta_{Asian}\neq 0$&$\surd$&$\beta_1>0,\beta_2>0,\beta_3<0$\\
1.2 Expected variation (second moment)&$\times$&Q5, $\beta_{Asian}\neq 0$&$\times$&$\sigma_{AR}^{II}\neq1$\\
1.3 Strategic channel&$\times$&Q2, $\beta_{Asian}\neq 0$&$\times$&$\beta_{Ivy}<0$\\
\midrule
\textbf{2. Taste-Based
Mechanisms}&&&&\\
\midrule
2.1 Friendly Support&$\surd$&Asian founders receive more donations&$\varnothing$&$\beta_1>0,\beta_2>0,\beta_3>=0$\\
2.2 Social Image&$\varnothing$&&$\varnothing$&\\
\midrule
\textbf{Amplifying Mechanisms}&&&&\\
\midrule
a. Attention Discrimination&$\varnothing$&&$\surd$&$\beta_1>0$ when $Y_{ij}$ is opening rates and email staying time.\\
b. Implicit Bias&\textcolor{red}{$\surd$ (against)}&Q1, $\beta_{Asian}\neq 0$&$\varnothing$&\\

\midrule
\textbf{3. Other Specific Mechanisms}&&&&\\
\midrule
3.1 Uninformative Email Behaviors&N/A&&$\times$&$\beta_1>0$ when $Y_{ij}$ is opening rates and email staying time.\\
3.2 Fishy Emails&N/A&&$\times$&$\beta_2<0$\\
\bottomrule
\end{tabular}}
 \end{center}
\begin{tablenotes}
\item \footnotesize \emph{Notes.} This table shows the mechanisms predicted by different racial discrimination theories and whether such mechanisms are supported by the empirical results from the correspondence test and the lab-in-field experiment or not. ``$\surd$" means such a mechanism is supported by the empirical evidence from the specific experiment. ``$\times$" means that such a mechanism is ruled out by the empirical evidence from the specific experiment. ``$\varnothing$" means that the experiment does not provide empirical evidence to support or rule out such a mechanism. The parameters used in the correspondence test theory predictions are from the following regressions: $Y_{ij}=\beta_0+\beta_1 AsianFounder{ij}+\beta_2 Ivy_{ij}+\beta_3 AsianFounder_{ij}\times Ivy_{ij}+\alpha_i +\epsilon_{ij}$ with pitch email fixed effect, where $Y_{ij}$ are the behavior measurements like the opening rate dummy, etc. $AsianFounder_{ij}$ and $Ivy_{ij}$ are indicators of being an Asian founder and graduating from Ivy League colleges. $\sigma_{AR}^{II}$ is the ratio of standard errors of Asian founders' unobservable characteristics and white founders' unobservable characteristics. I found bias towards Asian founders ($\beta_1>0$) in general in the correspondence test. Hence, all the theory predictions are to explain the reasons why investors prefer Asian founders starting in 04/2020. The parameters used in the lab-in-field theory predictions are from the following regressions: $V_{ij}=\beta_0+\beta_c Characteristics_{ijc}+\alpha_i+\epsilon_{ij}$ with evaluator fixed effect. $V_{ij}$ can be the evaluation of Q1(quality), Q2(collaboration likelihood), Q3(contact), Q4(investment) and Q5(risk). Please note that all the mechanisms can exist at the same time with some mechanisms dominating others in specific experimental settings.\\
\end{tablenotes}
\end{sidewaystable}
