# Supplementary material for: Discrimination in the Venture Capital Industry: Evidence from Field Experiments
Source: arXiv:2010.16084 source file (2022-08-14)
Supplement: Supplementary file 2 [file appendix_model.tex]

Assume that the quality of startup depends linearly and additively on two characteristics: $X^{I*}$ which includes standardized observable information in the pitch email; $X^{II}$ which includes unobservable characteristics of each startup. Let G=1 denote being a female founder and G=0 denote being a male founder. (Similar logic can also be applied to Asian founders and white founders.) Define $\gamma$ as an additional linear additive terms that reflects taste-based bias or belief-based bias (i.e. $E(X_F^{II})\neq E(X_M^{II})$ ) based on the founder' gender. Define $F$ as fund-level characteristics, which are normally distributed, independent of $X^{II}$, and follows the same distribution for female founders and male founders.\par

%%%%%%%%%%%%%%%%%%%%
%%% HS Critique %%%
%%%%%%%%%%%%%%%%%%%%
\subsection{Heckman's Critique}
Based on the model from \cite{neumark_detecting_2012}, the investor would open or reply to an email if a startup's perceived quality exceeds an internal threshold $c'(>0)$. Then the callback decisions (i.e. the email opening decision or email reply decision) for female and male founders are\par
\begin{eqnarray*}
T(P(X^{I*}, X_F^{II})|G=1)=1 \text{ if }\beta_1^{'}X^{I*}+X_F^{II}+\gamma^{'}+F>c'\\
T(P(X^{I*}, X_M^{II})|G=0)=1 \text{ if }\beta_1^{'}X^{I*}+X_M^{II}+F>c'\\
\end{eqnarray*}
where $X_F^{II}$ and $X_M^{II}$ are residuals. Assume that $X_F^{II}$ and $X_M^{II}$ are normaly distributed with zero means and standard deviations $\sigma_F^{II}$ and $\sigma_M^{II}$, and the distribution function $\Phi$, then the email opening probabilities are\par

\begin{center}
\begin{eqnarray*}
\text{open/reply emails if} X_F^{II}/\sigma_F^{II} >(c'-\beta_1^{'}X^{I*}-\gamma^{'})/\sigma_F^{II} \text{ where } \frac{X_F^{II}}{\sigma_F^{II}}\sim N(0,1)\\
 \text{(10)} \underbrace{Pr[T(P(X^{I*}, X_F^{II})|G=1)=1]}_\text{opening/reply probability for female}=1-\Phi[\frac{c'-\beta_1^{'}X^{I*}-\gamma^{'}}{\sigma_F^{II}}]=\Phi[\frac{-c'+\beta_1^{'}X^{I*}+\gamma^{'}}{\sigma_F^{II}}]\\
 \text{(10')}\underbrace{Pr[T(P(X^{I*}, X_M^{II})|G=0)=1]}_\text{opening/reply probability for male}=1-\Phi[\frac{c'-\beta_1^{'}X^{I*}}{\sigma_M^{II}}]=\Phi[\frac{-c'+\beta_1^{'}X^{I*}}{\sigma_M^{II}}]\\
\end{eqnarray*}
\end{center}

Without further assumption on $\sigma_F^{II}$ and $\sigma_M^{II}$, $\gamma$ is unidentified. The model mentioned above illustrates the Heckman's critique. In a correspondence test, $X_F^I$=$X_M^I=X^I$. Consider the situation where $\gamma'=0$ (no discrimination), but $Var(X_M^I)>Var(X_F^I)$ (i.e. the variance of male founders is larger than the variance of female founders)\par
\vspace{2cm}
\textbf{Case I:} When $X^{I*}$ is low, investors prefer male entrepreneurs (higher variance group) whose $Var(X_M^I)$ is higher. (spurious evidence of discrimination against women)\par

\begin{center}
\begin{eqnarray*}
\text{If}\quad \beta_I'X^{I*}<c', \underbrace{\Phi[\frac{-c'+\beta_1^{'}X^{I*}+\gamma^{'}}{\sigma_F^{II}}]}_\text{super negative}<\underbrace{\Phi[\frac{-c'+\beta_1^{'}X^{I*}}{\sigma_M^{II}}]}_\text{not very negative}
\end{eqnarray*}
\end{center}

\textbf{Case II:} When $X^I$ is high, investors prefer female entrepreneurs (lower variance group) whose $Var(X_F^I)$ is lower.\footnote{For example, in \cite{gornall_gender_2020}, $X^{I*}$ is set as high as possible in order to increase the response rate.} (spurious evidence of discrimination in favor of women)\par
\begin{center}
\begin{eqnarray*}
\text{If}\quad \beta_I'X^{I*}>c', \underbrace{\Phi[\frac{-c'+\beta_1^{'}X^{I*}+\gamma^{'}}{\sigma_F^{II}}]}_\text{super positive}>\underbrace{\Phi[\frac{-c'+\beta_1^{'}X^{I*}}{\sigma_M^{II}}]}_\text{not very positive}\\
\end{eqnarray*}
\end{center}
The HS Critique argument holds for symmetric distributions (\cite{heckman1998detecting}) and claims that even under ideal conditions, correspondence studies are uninformative about discrimination. The two cases mentioned above show that the relative variances of the unobservables interact with the level of quality set for the pitch email in the correspondence test. Therefore, it is important to check this potential bias from variances of unobservables to avoid spurious evidence of discrimination in favor of women.\par

\vspace{2mm}
Note that the Heckman's Critique comes from the nonlinear binary callback rates used in the correspondence test. It does not apply to the lab-in-field experiment where the outcome variables are continuous and linear.\\ (i.e. Rating=$\beta_1^{'}X^{I*}
+X_F^{II}+\gamma^{'}+F$ for female founders and Rating=$\beta_1^{'}X^{I*}+X_M^{II}+F$ for male founders.)

%%%%%%%%%%%%%%%%%%%%
%%% Neumark 2012 %%%
%%%%%%%%%%%%%%%%%%%%
\subsection{Correct Bias Using Neumark Model}
\cite{neumark_detecting_2012} model shows that when the correspondence test introduces meaning variation of quality that shift investors' response decisions, $\gamma$ can be identified. The intuition is that when a group has higher variance (i.e. male founders), the effect of its observable characteristics will be smaller. Therefore, checking how quality variation affects investors' callback decisions can help identify the relative variance of the unobservables, and in turn identify $\gamma$ (i.e. the bias parameter).\par 

\vspace{2mm}
The model has the following two assumptions: a). There are some startup characteristics (i.e. the education background in Experiment 1) in the study that affect perceived quality. b). $\beta_I$ is the same for female founders and male founders. (Such assumption cannot be tested in Experiment 1 setting because there is only one significant quality control, which is education background of the startup founder.)\par

\begin{center}
\begin{eqnarray*}
\text{Outcome difference}\quad  \underbrace{\Phi[\frac{-c'+\beta_1^{'}X^{I*}+\gamma^{'}}{\sigma_F^{II}}]}_\text{response rate for female founders}-\underbrace{\Phi[\frac{-c'+\beta_1^{'}X^{I*}}{\sigma_M^{II}}]}_\text{response rate for male founders}\\
\end{eqnarray*}
\end{center}
I can only identify the coefficients relative to the standard deviation of the unobservable, so I normalize the variance. Set $\sigma_M^{II}=1$ and $\sigma_F^{II}$ is then the variance of the observable for female founders relative to male founders and $\sigma_{FR}^{II}=\frac{\sigma_F^{II}}{\sigma_M^{II}}=\sigma_F^{II}$ after normalization.
\begin{center}
\begin{eqnarray*}
\text{ Outcome difference}\quad  (*)\underbrace{\Phi[\frac{-c'+\beta_1^{'}X^{I*}+\gamma^{'}}{\textcolor{orange}{\sigma_{FR}^{II}}}]}_\text{response rate for female founders}-\underbrace{\Phi[-c'+\beta_1^{'}X^{I*}]}_\text{response rate for male founders}\\
\end{eqnarray*}
\end{center}

(*) can be non-zero due to either (1) $\gamma'\neq 0$ or (2) $\sigma_{FR}\neq 1$, which makes the discrimination not identifiable.\par

\vspace{2mm}
To estimate $\frac{\beta_I}{\sigma_{BR}^{II}}$, $\beta_I$, and inferences on their ratio $\sigma_{BR}^{II}=\frac{\sigma_B^{II}}{\sigma_W^{II}}$, I can implement a heteroskedastic probit model which allows the variance of unobservable to vary with gender.\par

\vspace{2mm}
Define i as startup pitch email, define j as investor j. There is a latent variable for perceived quality relative to the threshold, assumed to be generated by

\begin{eqnarray*}
T(P_{ij*})=-c+\beta_I X_{ij}^{I*}+\gamma G_{i}+\epsilon_{ij}\\
\end{eqnarray*}

Assume $E(\epsilon_{ij})=0$ and var$(\epsilon_{ij})$=$[exp(\mu_\omega G_i)]^2$. $\mu$ is also normalized to 0. This model can be estimated via maximum likelihood and the observations are treated as clustered on investor level. Then the estimate of $exp(\omega)$ is equal to $\sigma_{BR}^{II}$.\par

\vspace{2mm}
\textbf{Assume that $\beta_I$ is the same for female and male in order to identify $\gamma$}\\
Observations on male founders identify:$-c$ and $\beta_I$\\
Observations on female founders identify:$\frac{(-c+\gamma)}{\underbrace{exp(\omega)}_{= \sigma_{FR}^{II}}}$ and $\frac{\beta_I}{\underbrace{exp(\omega)}_{= \sigma_{FR}^{II}}}$\\

The ratio of $\beta_I$ and $\frac{\beta_I}{\underbrace{exp(\omega)}_{= \sigma_{FR}^{II}}}$ can identify $exp(\omega)$  , which is equal to $\sigma_{FR}^{II}$.

With $c$ and $exp(\omega)$,  the expression of $\frac{(-c+\gamma)}{\underbrace{exp(\omega)}_{= \sigma_{FR}^{II}}}$ identifies $\gamma$. If we allow statistical discrimination, which means that $E(X_F^{II})-E(X_M^{II})=\mu_{FW}^{II}\neq 0$, then what we identify is $\gamma+\mu_{FW}^{II}$ rather than $\gamma$. This is the combination of taste discrimination and the statistical discrimination.

\vspace{2mm}
If $\sigma_{FR}^{II}=1$, then there is no bias from differences in the distribution of unobservabes. If $\sigma_{FR}^{II}\neq1$, but we had some evidence on how the level of standardization $X^{I*}$ compares to the relevant startup pitch emails, we could determine the direction of bias.\footnote{Stata Code: dprobit, vce(cluster)}

\vspace{2mm}
\subsection{Extension of Neumark Model by Adding Strategic Channel}
In the \cite{neumark_detecting_2012} model described in B.2, the higher the startup perceived quality, the more likely the investor will open this email. However, if some emails are too good (``overqualified"), investors may not want to look at them. Although such mechanism does not play an important role in Experiment 1 setting because better education background positively affects investors' response. Such extra mechanism can be added in the previous model by assuming the following non-monotonic hiring rule:
\begin{eqnarray*}
c_2'>\beta_1^{'}X^{I*}+X_F^{II}+\gamma^{'}+F>c_1'
\end{eqnarray*}
Use the following MLE method to estimate the model:\bigskip
\begin{center}
\begin{eqnarray*}
T_{ij}=&1\{c_1'<\beta X_1^{I*}+X_2^{II}+\gamma' G +\epsilon_{ij}<c_2'\}\\
T_{ij}=&1\{(c_1'-X_1^{I*}-\gamma' G)/\sigma_B<X_2^{II}+\epsilon_{ij}<(c_2'-X_1^{I*}-\gamma' G)/\sigma_B\}\\
\prod_{i=1}^{n}(\Phi(\frac{(c_2'-X_1^{I*}-\gamma')}{\sigma_B^F})-&\Phi(\frac{(c_1'-X_1^{I*}-\gamma')}{\sigma_B^F}))^{T_{i\in F,j}=1}(\Phi(\frac{(c_2'-X_1^{I*})}{\sigma_B^M})-\Phi(\frac{(c_1'-X_1^{I*})}{\sigma_B^M}))^{T_{i\in M,j}=1}\\
\end{eqnarray*}
\end{center}
Such extension is not trivial since it is currently a non-monotonic crossing threshold model and it is hard to non-parametrically estimate such models. (see \cite{lee2018identifying})
